# Supplementary material for: Autonomous Drone Racing with Deep Reinforcement Learning
Source: arXiv:2103.08624 source file (2021-08-02)
Supplement: Supplementary file 1 [file appendix.tex]

\subsection*{Supplementary Materials}

\subsubsection{Gate Displacement}

\begin{table}[!thp]
\caption{Definition of gate-specific perturbation bounds for Alpha Pilot track. \TODO{this seems redundant if used together with Fig. 6. I like the figure more.}}
\label{tab:gate-displacements}
\begin{center}
\begin{tabular}{| c | c | c | c | c |}
\hline
Gate & $\Delta{x}$ [m]  & $\Delta{y}$ [m]  & $\Delta{z}$ [m] & $\Delta{\alpha} [\circ]$  \\ \hline
1    & [-7.0, 7.0]  & [-7.0, 7.0]   & [-5.0, 5.0] & [-5.0, 5.0]  \\ \hline
2    & [-1.0, 1.0]  & [-1.0, 1.0]   & [-5.0, 5.0] & [-45.0, 45.0]  \\ \hline
3    & [-3.0, 3.0]  & [-3.0, 3.0]   & [-3.0, 3.0] & [-5.0, 5.0]  \\ \hline
4    & [-4.5, 4.5]  & [-4.5, 4.5]   & [-3.0, 3.0] & [-5.0, 5.0]  \\ \hline
5    & [-2.5, 2.5]  & [-2.5, 2.5]   & [-3.0, 3.0] & [-5.0, 5.0]  \\ \hline
6    & [-1.0, 1.0]  & [-1.0, 1.0]   & [-1.0, 1.0] & [-5.0, 5.0]  \\ \hline
7    & [-2.5, 2.5]  & [-2.5, 2.5]   & [-1.0, 1.0] & [-5.0, 5.0]  \\ \hline
8    & [-1.0, 1.0]  & [-1.0, 1.0]   & [-1.0, 1.0] & [-5.0, 5.0]  \\ \hline
9    & [-4.5, 4.5]  & [-4.5, 4.5]   & [-3.0, 3.0] & [-20.0, 20.0]  \\ \hline
10    & [-7.0, 7.0]  & [-7.0, 7.0]   & [-5.0, 5.0] & [-5.0, 5.0]  \\ \hline
11    & [-4.5, 4.5]  & [-4.5, 4.5]   & [-5.0, 5.0] & [-5.0, 5.0]  \\ \hline
\end{tabular}
\end{center}
\end{table}

\subsubsection{Quadrotor Configurations}

\subsubsection{Policy Training}
